# Supplementary material for: A Smartphone based Application for Skin Cancer Classification Using Deep Learning with Clinical Images and Lesion Information
Source: arXiv:2104.14353 source file (2021-04-28)
Supplement: Supplementary file 1 [file appendix.tex]

% 88888888888888888888888       BACC        888888888888888888888888

\begin{table*}[htbp]
\caption{Best setup simulations for BACC}
\centering
\begin{tabular}{|c|c|c|c|c|c|}
\hline
& \multicolumn{5}{c|}{Beta} \\ \hline
C & {1} & {3} & {5} & {7} & {10} \\ \hline
1 & {62.66 $\pm$ 9.30} & {89.44 $\pm$ 3.48} & {90.57 $\pm$ 6.61} & {86.19 $\pm$ 3.21} & {80.48 $\pm$ 11.75} \\ \hline
2 & {72.25 $\pm$ 12.97} & {89.23 $\pm$ 12.66} & {82.70 $\pm$ 12.70} & {83.54 $\pm$ 7.74} & {84.09 $\pm$ 8.02} \\ \hline
3 & {75.99 $\pm$ 13.31} & {91.79 $\pm$ 5.56} & {83.79 $\pm$ 9.31} & {89.00 $\pm$ 3.64} & {74.72 $\pm$ 17.19} \\ \hline
4 & {74.81 $\pm$ 5.29} & {89.91 $\pm$ 9.98} & {93.02 $\pm$ 2.12} & {81.84 $\pm$ 7.10} & {77.75 $\pm$ 10.55} \\ \hline
5 & {68.17 $\pm$ 12.65} & {87.21 $\pm$ 5.99} & {92.32 $\pm$ 2.89} & {84.97 $\pm$ 9.79} & {85.12 $\pm$ 10.29} \\ \hline
\end{tabular}
\label{tab_bacc_bsp}
\end{table*}

% % 88888888888888888888888       ACC        888888888888888888888888

% \begin{table*}[htbp]
% \centering
% \caption{Best setup simulations for ACC}
% \begin{tabular}{|c|l|c|c|c|c|}
% \hline
% & \multicolumn{5}{c|}{Beta} \\ \hline
% C & {1} & {3} & {5} & {7} & {10} \\ \hline
% 1 & {97.10 $\pm$ 0.43} & {90.24 $\pm$ 9.32} & {84.45 $\pm$ 12.78} & {83.96 $\pm$ 5.00} & {78.26 $\pm$ 10.05} \\ \hline
% 2 & {97.01 $\pm$ 1.07} & {95.17 $\pm$ 3.68} & {85.22 $\pm$ 14.08} & {78.84 $\pm$ 10.35} & {79.90 $\pm$ 8.96} \\ \hline
% 3 & {96.23 $\pm$ 1.20} & {94.78 $\pm$ 2.98} & {79.32 $\pm$ 18.37} & {78.74 $\pm$ 7.04} & {53.82 $\pm$ 35.70} \\ \hline
% 4 & {96.62 $\pm$ 1.18} & {93.82 $\pm$ 4.81} & {89.18 $\pm$ 4.79} & {70.24 $\pm$ 12.52} & {75.65 $\pm$ 15.65} \\ \hline
% 5 & {97.10 $\pm$ 1.37} & {88.60 $\pm$ 5.85} & {87.83 $\pm$ 6.06} & {92.27 $\pm$ 3.98} & {73.91 $\pm$ 21.37} \\ \hline
% \end{tabular}
% \label{tab_acc_bsp}
% \end{table*}

% 88888888888888888888888       PR        888888888888888888888888

\begin{table*}[htbp]
\caption{Best setup simulations for PR}
\centering
\begin{tabular}{|c|c|c|c|c|c|}
\hline
& \multicolumn{5}{c|}{Beta} \\ \hline
C & {1} & {3} & {5} & {7} & {10} \\ \hline
1 & {63.33 $\pm$ 37.12} & {38.28 $\pm$ 18.97} & {22.81 $\pm$ 7.96} & {17.73 $\pm$ 6.34} & {14.78 $\pm$ 10.41} \\ \hline
2 & {55.09 $\pm$ 22.17} & {58.64 $\pm$ 28.25} & {24.42 $\pm$ 15.18} & {16.35 $\pm$ 7.79} & {15.62 $\pm$ 5.44} \\ \hline
3 & {47.02 $\pm$ 17.81} & {44.28 $\pm$ 18.43} & {20.77 $\pm$ 11.45} & {15.65 $\pm$ 6.87} & {14.34 $\pm$ 11.53} \\ \hline
4 & {61.55 $\pm$ 24.66} & {50.67 $\pm$ 28.65} & {27.07 $\pm$ 10.14} & {11.95 $\pm$ 5.99} & {12.99 $\pm$ 6.44} \\ \hline
5 & {63.33 $\pm$ 30.55} & {27.16 $\pm$ 13.20} & {25.03 $\pm$ 9.05} & {31.72 $\pm$ 10.0} & {19.23 $\pm$ 11.75} \\ \hline
\end{tabular}
\label{tab_pr_bsp}
\end{table*}

% 88888888888888888888888       REC        888888888888888888888888

\begin{table*}[htbp]
\caption{Best setup simulations for REC}
\centering
\begin{tabular}{|c|c|c|c|c|c|}
\hline
\cline{1-5}
C & {1} & {3} & {5} & {7} & {10} \\ \hline
1 & {25.71 $\pm$ 18.95} & {88.57 $\pm$ 10.69} & {97.14 $\pm$ 5.72} & {88.57 $\pm$ 5.72} & {82.86 $\pm$ 27.70} \\ \hline
2 & {45.72 $\pm$ 26.18} & {82.86 $\pm$ 27.70} & {80.0 $\pm$ 26.50} & {88.57 $\pm$ 22.86} & {88.57 $\pm$ 22.86} \\ \hline
3 & {54.29 $\pm$ 27.70} & {88.57 $\pm$ 10.69} & {88.57 $\pm$ 10.69} & {100.00 $\pm$ 0.00} & {97.14 $\pm$ 5.72} \\ \hline
4 & {51.43 $\pm$ 11.43} & {85.71 $\pm$ 22.13} & {97.14 $\pm$ 5.72} & {94.28 $\pm$ 7.00} & {80.00 $\pm$ 26.50} \\ \hline
5 & {37.14 $\pm$ 24.91} & {85.71 $\pm$ 15.65} & {97.14 $\pm$ 5.72} & {77.14 $\pm$ 23.21s} & {97.14 $\pm$ 5.72} \\ \hline
\end{tabular}
\label{tab_rec_bsp}
\end{table*}

\begin{table*}[htbp]
\caption{The beta with and without clinical information}
\begin{center}
\begin{tabular}{|c|c|c|c|c|}
\hline
\multirow[c]{2}{*}{\textbf{Beta}} & \multicolumn{4}{|c|}{\textbf{Metrics}} \\
\cline{2-5}
& \textbf{\textit{BACC}} & \textbf{\textit{ACC}} & \textbf{\textit{PR}}& \textbf{\textit{REC}} \\
\hline
% ---------------------------------------------------------------------------------------
{1} & {77.37 $\pm$ 13.84} & {96.23 $\pm$ 1.63} & {49.56 $\pm$ 23.21} & {57.14 $\pm$ 28.57} \\
\cline{1-5}
{3} & {78.83 $\pm$ 14.62} & { 93.72 $\pm$ 2.86} & {31.34 $\pm$ 14.59} & {62.86 $\pm$ 30.77} \\
\cline{1-5}
{5} & {82.92 $\pm$ 8.86} & {88.31 $\pm$ 5.61} & {22.25 $\pm$ 9.75} & {77.14 $\pm$ 17.14} \\
\cline{1-5}
{7} & {87.74 $\pm$ 4.03} & {86.96 $\pm$ 6.60} & {22.66 $\pm$ 8.29} & {88.57 $\pm$ 10.69} \\
\cline{1-5}
{10} & { 87.41 $\pm$ 6.96} & {88.99 $\pm$ 2.98} & {22.45 $\pm$ 4.41} & {85.71 $\pm$ 15.65} \\
% ---------------------------------------------------------------------------------------
\hline
\end{tabular}
\label{tab_beta_sem_dados}
\end{center}
\end{table*}
